# Supplementary material for: Learning Hierarchical Shape Segmentation and Labeling from Online Repositories
Source: arXiv:1705.01661 source file (2017-05-04)
Supplement: Supplementary file 1 [file supp.tex]

\begin{table}
\caption{\label{tab:labelfrequency} Tags and their frequency (percent of shapes that have a scene node, i.e. part, labeled with the corresponding tag) in the raw shapenet dataset.}
\centering
  \begin{tabular}{|l|l|c|c||l|c|c| }
  \hline
    \textbf{Category} & \textbf{Part}  & \textbf{Input} & \textbf{Output} & \textbf{Part}  & \textbf{Input} & \textbf{Output} \\ \hline
    \multirow{2}{*}{Airplane} & Wing  & 5.87\% & 95.68\% & Engine  & 5.48\% & 77.41\% \\ \hline
    & Body & 2.25\% & 98.01\% & Tail & 1.48\% & 98.67\% \\ \hline
    \multirow{2}{*}{Motorbike} & Seat  & 23.49\% & 89.58\% & Engine  & 21.71\% & 62.50\% \\ \hline
    & Handle & 8.90\% & 92.71\% & Gastank & 14.59\% & 78.13\% \\ \hline
    & Exhaust & 1.78\% & 86.46\% & Wheel & 41.64\% & 100.00\% \\ \hline
  \end{tabular}
\end{table}
